# Supplementary material for: On the characteristic features of ionization in QED environments
Source: arXiv:2203.06050 source file (2022-05-06)
Supplement: Supplementary file 1 [file Supplementary_Material.pdf]

# Supplementary Material: On the characteristic features of ionization in QED environments

Rosario Roberto Riso[1], Tor S. Haugland[1], Enrico Ronca[2], and Henrik Koch[1,3]

[1]Department of Chemistry, Norwegian University of Science and Technology, 7491 Trondheim, Norway
[2]Istituto per i Processi Chimico Fisici del CNR (IPCF-CNR), Via G. Moruzzi, 1, 56124, Pisa, Italy
[3]Scuola Normale Superiore, Piazza dei Cavalieri 7, 56126 Pisa, Italy

## 1 Definition of the bath orbital in optical cavities

A straightforward generalization of CC techniques to treat ionization potentials can be performed defining a bath orbital $\nu$ such that:

$$h_{\nu x} = d_{\nu x} = 0 \;\; \forall x \qquad g_{\nu xyz} = 0 \;\; \forall x,\; y\; z; \tag{1}$$

and then diagonalizing the Jacobian submatrix that excites to the free electron orbital. This is equivalent to having an electron that is not interacting with the cavity. However, this kind of approach leads to non-origin invariant ionization energies for charged molecules as we will discuss in the following. At the QED-CCSD-1 level, a general Jacobian matrix element between two one electron excitations involving the bath orbital $\nu$ is given by

$$\begin{aligned}\langle HF,0|\, i^\dagger_\sigma \nu_\sigma \left[e^{-T} H e^{T}, \nu^\dagger_\sigma j_\sigma\right] |HF,0\rangle = F_{ji} + \sum_a t^a_i F_{ai} \\ + \sum_{la} L_{jila} t^a_l + \sum_{lab} L_{jalb}(t^{ab}_{il} - t^a_i t^b_l) - \alpha \sum_a (\mathbf{d}\cdot\boldsymbol{\epsilon})_{ja} s^a_i,\end{aligned} \tag{2}$$

where $L_{pqrs}$ is defined as:

$$\begin{aligned}L_{pqrs} =& 2g_{pqrs} - g_{psrq} + 2(\mathbf{d}\cdot\boldsymbol{\epsilon})_{pq}(\mathbf{d}\cdot\boldsymbol{\epsilon})_{rs} \\ & -(\mathbf{d}\cdot\boldsymbol{\epsilon})_{ps}(\mathbf{d}\cdot\boldsymbol{\epsilon})_{rq},\end{aligned} \tag{3}$$

and $F_{pq}$ is the Fock matrix. Since $\mathbf{F}$ has been diagonalized in the reference calculation, Eq. 2 is equal to:

$$\begin{aligned}\langle HF,0|\, i^\dagger_\sigma \nu_\sigma \left[e^{-T} H e^{T}, \nu^\dagger_\sigma j_\sigma\right] |HF,0\rangle = \epsilon_j \delta_{ij} \\ + \sum_{la} L_{jila} t^a_l + \sum_{lab} L_{jalb}(t^{ab}_{il} - t^a_i t^b_l) - \alpha \sum_a (\mathbf{d}\cdot\boldsymbol{\epsilon})_{ja} s^a_i.\end{aligned} \tag{4}$$

The molecular dipole operator is

$$\mathbf{d}_{pq} = \mathbf{d}^e_{pq} + \frac{\mathbf{d}^N}{N_e}\delta_{pq}, \tag{5}$$

where $\mathbf{d}^e$ is the electronic dipole while $\mathbf{d}^N$ is the nuclear dipole. If the origin is shifted by a quantity $\mathbf{a}$ the dipole changes to

$$(\mathbf{d}\cdot\boldsymbol{\epsilon})_{pq} \longrightarrow (\mathbf{d}\cdot\boldsymbol{\epsilon})_{pq} + \frac{Q_{tot}}{N_e}(\mathbf{a}\cdot\boldsymbol{\epsilon})\delta_{pq}, \tag{6}$$

where $N_e$ is the number of electrons and $Q_{tot}$ is the total charge of the system. Therefore, the Jacobian in Eq. 4 is not origin invariant and upon displacement its elements transform as:

$$\langle HF,0|\, i^\dagger_\sigma \nu_\sigma \left[e^{-T}He^{T}, \nu^\dagger_\sigma j_\sigma\right] |HF,0\rangle = \epsilon_j\delta_{ij} + \sum_{la} L_{jila}t^a_l + \sum_{lab} L_{jalb}(t^{ab}_{il} - t^a_i t^b_l) - \alpha\sum_a (\mathbf{d}\cdot\boldsymbol{\epsilon})_{ja}s^a_i$$
$$+ \lambda^2\delta_{ij}\left(2(\mathbf{a}\cdot\boldsymbol{\epsilon})\sum_{ka}(\mathbf{d}\cdot\boldsymbol{\epsilon})_{ka}t^a_k - (\mathbf{d}\cdot\boldsymbol{\epsilon})_{ii}(\mathbf{a}\cdot\boldsymbol{\epsilon})\right) - \lambda^2(\mathbf{a}\cdot\boldsymbol{\epsilon})\sum_a(\mathbf{d}\cdot\boldsymbol{\epsilon})_{ja}t^a_i - \delta_{ij}\frac{\lambda^2(\mathbf{a}\cdot\boldsymbol{\epsilon})^2}{2}, \tag{7}$$

We point out that the first lines of Eq. 7 is equal to Eq. 4. The non-origin invariance of Eq.2 is surprising since the excitation energies computed using EOM-QED-CCSD-1

$$\langle \mu, n|\, e^{-T}\left[H, \tau_\nu\left(b^\dagger\right)^m\right] e^{T}|HF,0\rangle, \tag{8}$$

are instead origin invariant. In passing, we also note that the same relationships holds for the following two quantities

$$\begin{aligned}\langle HF,0|\, E_{ia}HE_{ai}\,|HF,0\rangle &\longrightarrow \text{origin invariant}\\ \langle HF,0|\, E_{i\nu}HE_{\nu i}\,|HF,0\rangle &\longrightarrow \text{non origin invariant.}\end{aligned} \tag{9}$$

To better understand the difference between Eq. 8 and Eq. 7 we explicitly show here that the Jacobian element between one electron excitations to orbitals $a$ and $b$ from the occupied orbitals $i$ and $j$:

$$\langle HF,0|\, E_{ia}\left[e^{-T}He^{T}, E_{bj}\right] |HF,0\rangle, \tag{10}$$

where $\alpha$ and $\sigma$ over the spin states, is origin invariant. This quantity is equal to:

$$\langle HF,0|\, E_{ia}\left[e^{-T}He^{T}, E_{bj}\right] |HF,0\rangle = \delta_{ij}F_{ab} - \delta_{ab}F_{ji} - 2\beta d_{ji}d_{ab} + \lambda^2\sum_c(2d_{ac}d_{jb} - d_{jc}d_{ab})t^c_i$$
$$+\lambda^2\sum_k(d_{ji}d_{kb} - 2d_{ki}d_{jb})t^a_k + \lambda^2\delta_{ij}\sum_{kc}(2d_{kc}d_{ab} - d_{ac}d_{kb})t^c_k - \lambda^2\delta_{ab}\sum_{kc}(2d_{kc}d_{ji} - d_{ki}d_{jc})t^c_k,$$

containing origin dependent terms that however mutually cancel out. The main difference between Eq. 4 and Eq. 8 is that the non origin invariant contributions from $(\mathbf{d}\cdot\boldsymbol{\epsilon})_{jj}$ are not canceled by opposite contributions coming from $(\mathbf{d}\cdot\boldsymbol{\epsilon})_{\nu\nu}$ if the definition in Eq. 1 is adopted.
In particular, if the molecule is displaced by a vector $\mathbf{a}$, $(\mathbf{d}\cdot\boldsymbol{\epsilon})_{\nu\nu}$ should behave like all the dipole elements from the other orbitals:

$$(\mathbf{d}\cdot\boldsymbol{\epsilon})_{\nu\nu} \rightarrow (\mathbf{d}\cdot\boldsymbol{\epsilon})_{\nu\nu} \qquad \text{Neutral molecule,} \tag{11}$$

$$(\mathbf{d}\cdot\boldsymbol{\epsilon})_{\nu\nu} \rightarrow (\mathbf{d}\cdot\boldsymbol{\epsilon})_{\nu\nu} + (\mathbf{a}\cdot\boldsymbol{\epsilon})\frac{Q_{tot}}{N_e} \quad \text{Charged molecule,} \tag{12}$$

property that is not respected if the dipole is equal to zero as in Eq. 1. In Eq.12 $Q_{tot}$ is the total charge of the system and $N_e$ is the number of electrons. In this paper we adopt the following choice for the free part of the dipole operator:

$$(\mathbf{d}\cdot\boldsymbol{\epsilon})_{\nu\nu} = \frac{\sqrt{2E_{free}}}{\lambda} - \frac{\sum_\alpha Z_\alpha(\mathbf{r}_\alpha\cdot\boldsymbol{\epsilon})}{\sum_\alpha Z_\alpha} + \frac{\sum_\alpha Z_\alpha(\mathbf{r}_\alpha\cdot\boldsymbol{\epsilon})}{N_e} \tag{13}$$

where $E_{\text{free}}$ is the energy of the free electron while $Z_\alpha$ and $\mathbf{r}_\alpha$ are the charge and the position of the nucleus $\alpha$ respectively. Analyzing in detail the various terms we observe that the last contribution in Eq. 13 is represented by the nuclear contribution to the molecular dipole. The electronic part of the dipole instead is equal to:

$$(\mathbf{d}^e\cdot\boldsymbol{\epsilon})_{\nu\nu} = -\int \phi^*_\nu(\mathbf{x}-\mathbf{R})(\mathbf{x}\cdot\boldsymbol{\epsilon})\phi_\nu(\mathbf{x}-\mathbf{R})d^3x \tag{14}$$

where $\mathbf{R}$ is the position of the nuclear center of charge. The free electron orbital can be thought of as a very diffuse orbital centered at the nuclei's center of charge. In this situation, the integral in Eq. 14 equals to

$$(\mathbf{d}^e\cdot\boldsymbol{\epsilon})_{\nu\nu} = -\int \phi^*_\nu(\mathbf{x})(\mathbf{x}\cdot\boldsymbol{\epsilon})\phi_\nu(\mathbf{x})d^3x - \frac{\sum_\alpha Z_\alpha(\mathbf{r}_\alpha\cdot\boldsymbol{\epsilon})}{\sum_\alpha Z_\alpha} \tag{15}$$

where now the integral value can be fixed to return the correct free orbital energy at the SC-QED-HF level:

$$(\mathbf{d}\cdot\boldsymbol{\epsilon})_{\nu\nu} = \frac{\sqrt{2E_{free}}}{\lambda} - \frac{\sum_\alpha Z_\alpha(\mathbf{r}_\alpha\cdot\boldsymbol{\epsilon})}{\sum_\alpha Z_\alpha} + \frac{\sum_\alpha Z_\alpha(\mathbf{r}_\alpha\cdot\boldsymbol{\epsilon})}{N_e}. \tag{16}$$

If the definition in Eq. 16 is adopted, the ionization energies become origin invariant. In addition, we notice that using Eq. 13, the following quantity also becomes origin invariant:

$$\langle HF,0|\, E_{i\nu} H E_{\nu i}\, |HF,0\rangle = E_{QED-HF} + \frac{\lambda^2}{2}(\mathbf{d}\cdot\boldsymbol{\epsilon})^2_{\nu\nu} - \epsilon_i - \lambda^2(\mathbf{d}\cdot\boldsymbol{\epsilon})_{ii}(\mathbf{d}\cdot\boldsymbol{\epsilon})_{\nu\nu}, \tag{17}$$

both for charged and neutral systems.

## 2 Results for the full molecular set

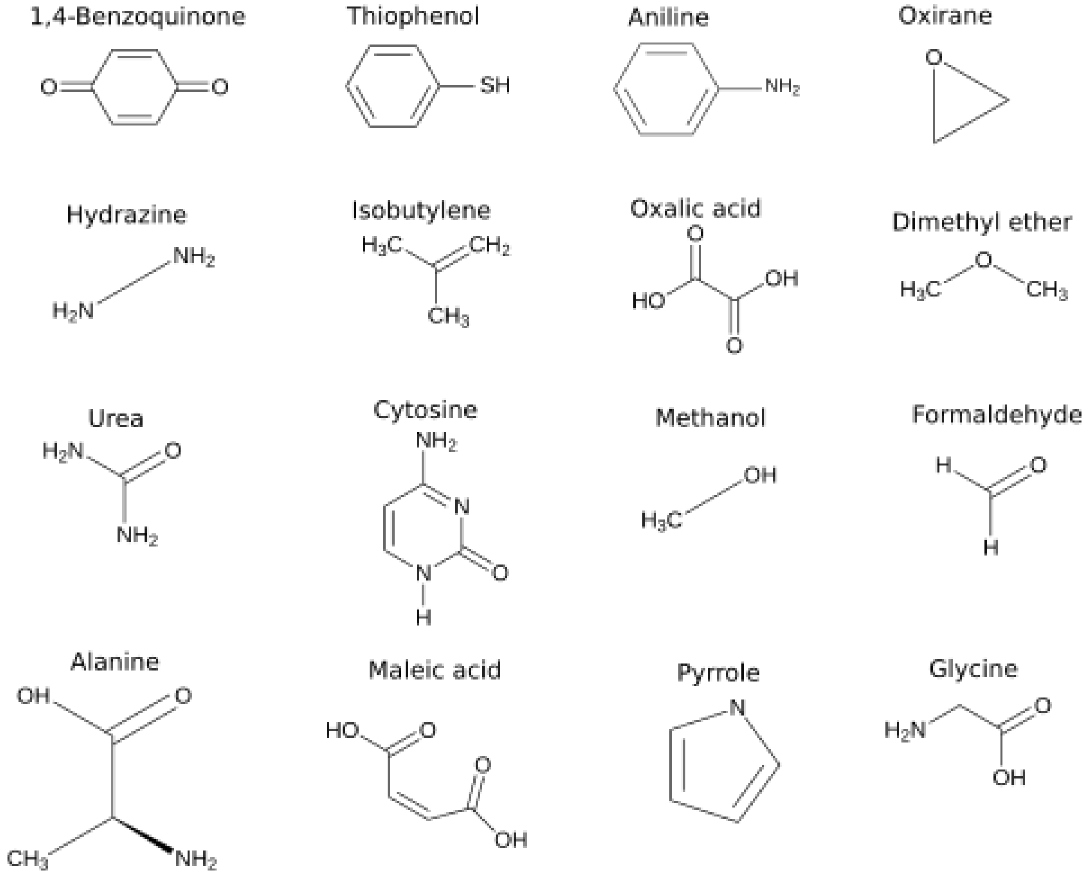


Figure 1: Investigated set of molecules.

In this section we report the results relative to the dependence of the IPs on $\lambda$ (at fixed $\omega_c = 13.6eV$) and $\omega_c$ (at fixed $\lambda = 0.05a.u.$) for the full set of molecules showed in Fig. 1. The field polarization is always along the z axis and the molecular geometries are reported in the repository found at the link: "https://doi.org/10.5281/zenodo.6498001 ". The excitation energies are reported in eV.

| $\lambda$ | SC-QED-HF | EOM-QED-CC | F-SC-QED-HF | F-EOM-QED-CC |
|---|---|---|---|---|
| 0.005 | 11.100 | 9.788 | 11.107 | 9.788 |
| 0.01 | 11.099 | 9.787 | 11.125 | 9.787 |
| 0.015 | 11.098 | 9.787 | 11.157 | 9.787 |
| 0.02 | 11.096 | 9.785 | 11.201 | 9.786 |
| 0.025 | 11.094 | 9.784 | 11.257 | 9.785 |
| 0.03 | 11.091 | 9.781 | 11.326 | 9.785 |
| 0.035 | 11.089 | 9.779 | 11.407 | 9.785 |
| 0.04 | 11.085 | 9.777 | 11.500 | 9.787 |
| 0.045 | 11.081 | 9.774 | 11.605 | 9.789 |
| 0.05 | 11.077 | 9.771 | 11.722 | 9.792 |

Table 1: Dispersion of the IPs with $\lambda$ for benzoquinone obtained using SC-QED-HF and F-SC-QED-HF and EOM-QED-CC and F-EOM-QED-CC

| $\lambda$ | SC-QED-HF | EOM-QED-CC | F-SC-QED-HF | F-EOM-QED-CC |
|---|---|---|---|---|
| 0.005 | 8.681 | 7.986 | 8.688 | 7.986 |
| 0.01 | 8.680 | 7.986 | 8.707 | 7.986 |
| 0.015 | 8.679 | 7.984 | 8.739 | 7.985 |
| 0.02 | 8.678 | 7.983 | 8.783 | 7.984 |
| 0.025 | 8.676 | 7.981 | 8.841 | 7.983 |
| 0.03 | 8.674 | 7.979 | 8.911 | 7.982 |
| 0.035 | 8.671 | 7.976 | 8.993 | 7.982 |
| 0.04 | 8.668 | 7.973 | 9.087 | 7.983 |
| 0.045 | 8.664 | 7.969 | 9.194 | 7.984 |
| 0.05 | 8.660 | 7.966 | 9.314 | 7.987 |

Table 2: Dispersion of the IPs with $\lambda$ for cytosine obtained using SC-QED-HF and F-SC-QED-HF and EOM-QED-CC and F-EOM-QED-CC

| $\omega_c$ | SC-QED-HF | EOM-QED-CC | F-SC-QED-HF | F-EOM-QED-CC |
|---|---|---|---|---|
| 13.6 | 8.286 | 8.047 | 8.319 | 8.048 |
| 5.804 | 8.282 | 8.044 | 8.908 | 8.047 |
| 2.477 | 8.280 | 8.042 | 8.976 | 8.056 |
| 1.057 | 8.279 | 8.041 | 9.008 | 8.109 |
| 0.451 | 8.278 | 8.041 | 9.027 | 8.227 |
| 0.192 | 8.278 | 8.041 | 9.039 | 8.357 |
| 0.082 | 8.278 | 8.041 | 9.044 | 8.461 |
| 0.035 | 8.278 | 8.041 | 9.047 | 8.533 |
| 0.015 | 8.278 | 8.041 | 9.048 | 8.582 |
| 0.006 | 8.278 | 8.041 | 9.049 | 8.615 |
| 0.003 | 8.278 | 8.041 | 9.049 | 8.636 |

Table 3: Dispersion of the IPs with $\omega_c$ for thiophenol obtained using SC-QED-HF and F-SC-QED-HF and EOM-QED-CC and F-EOM-QED-CC

| $\lambda$ | SC-QED-HF | EOM-QED-CC | F-SC-QED-HF | F-EOM-QED-CC |
|---|---|---|---|---|
| 0.005 | 12.117 | 10.134 | 12.119 | 10.134 |
| 0.01 | 12.116 | 10.133 | 12.125 | 10.133 |
| 0.015 | 12.114 | 10.132 | 12.134 | 10.132 |
| 0.02 | 12.111 | 10.130 | 12.148 | 10.130 |
| 0.025 | 12.108 | 10.127 | 12.164 | 10.129 |
| 0.03 | 12.103 | 10.124 | 12.183 | 10.128 |
| 0.035 | 12.098 | 10.120 | 12.206 | 10.126 |
| 0.04 | 12.093 | 10.116 | 12.231 | 10.125 |
| 0.045 | 12.086 | 10.111 | 12.258 | 10.125 |
| 0.05 | 12.078 | 10.106 | 12.288 | 10.126 |

Table 4: Dispersion of the IPs with $\lambda$ for oxirane obtained using SC-QED-HF and F-SC-QED-HF and EOM-QED-CC and F-EOM-QED-CC

| $\lambda$ | SC-QED-HF | EOM-QED-CC | F-SC-QED-HF | F-EOM-QED-CC |
|---|---|---|---|---|
| 0.005 | 7.566 | 7.268 | 7.568 | 7.268 |
| 0.01 | 7.565 | 7.268 | 7.574 | 7.268 |
| 0.015 | 7.564 | 7.267 | 7.584 | 7.267 |
| 0.02 | 7.562 | 7.265 | 7.598 | 7.265 |
| 0.025 | 7.559 | 7.262 | 7.616 | 7.264 |
| 0.03 | 7.556 | 7.260 | 7.636 | 7.264 |
| 0.035 | 7.553 | 7.257 | 7.660 | 7.263 |
| 0.04 | 7.549 | 7.253 | 7.687 | 7.263 |
| 0.045 | 7.544 | 7.249 | 7.717 | 7.264 |
| 0.05 | 7.539 | 7.244 | 7.749 | 7.266 |

Table 5: Dispersion of the IPs with $\lambda$ for aniline obtained using SC-QED-HF and F-SC-QED-HF and EOM-QED-CC and F-EOM-QED-CC

| $\omega_c$ | SC-QED-HF | EOM-QED-CC | F-SC-QED-HF | F-EOM-QED-CC |
|---|---|---|---|---|
| 13.6 | 7.546 | 7.250 | 7.581 | 7.250 |
| 5.804 | 7.542 | 7.247 | 7.621 | 7.250 |
| 2.477 | 7.540 | 7.245 | 7.714 | 7.259 |
| 1.057 | 7.538 | 7.244 | 7.871 | 7.312 |
| 0.451 | 7.538 | 7.243 | 8.029 | 7.431 |
| 0.192 | 7.537 | 7.243 | 8.128 | 7.563 |
| 0.082 | 7.537 | 7.243 | 8.178 | 7.667 |
| 0.035 | 7.537 | 7.243 | 8.200 | 7.741 |
| 0.015 | 7.537 | 7.243 | 8.210 | 7.791 |
| 0.006 | 7.537 | 7.243 | 8.214 | 7.823 |
| 0.003 | 7.537 | 7.243 | 8.217 | 7.845 |

Table 6: Dispersion of the IPs with $\omega_c$ for aniline obtained using SC-QED-HF and F-SC-QED-HF and EOM-QED-CC and F-EOM-QED-CC

| $\omega_c$ | SC-QED-HF | EOM-QED-CC | F-SC-QED-HF | F-EOM-QED-CC |
|---|---|---|---|---|
| 13.6 | 9.329 | 9.244 | 9.673 | 9.245 |
| 5.804 | 9.324 | 9.239 | 9.761 | 9.242 |
| 2.477 | 9.320 | 9.236 | 9.813 | 9.251 |
| 1.057 | 9.318 | 9.235 | 9.839 | 9.303 |
| 0.451 | 9.317 | 9.234 | 9.855 | 9.422 |
| 0.193 | 9.317 | 9.234 | 9.864 | 9.553 |
| 0.082 | 9.317 | 9.234 | 9.869 | 9.657 |
| 0.035 | 9.317 | 9.234 | 9.871 | 9.730 |
| 0.015 | 9.317 | 9.234 | 9.872 | 9.779 |
| 0.006 | 9.317 | 9.234 | 9.873 | 9.812 |
| 0.003 | 9.317 | 9.234 | 9.873 | 9.834 |

Table 7: Dispersion of the IPs with $\omega_c$ for isobutylene obtained using SC-QED-HF and F-SC-QED-HF and EOM-QED-CC and F-EOM-QED-CC

| $\lambda$ | SC-QED-HF | EOM-QED-CC | F-SC-QED-HF | F-EOM-QED-CC |
|---|---|---|---|---|
| 0.005 | 12.425 | 10.415 | 12.429 | 10.415 |
| 0.01 | 12.424 | 10.415 | 12.441 | 10.415 |
| 0.015 | 12.423 | 10.414 | 12.461 | 10.414 |
| 0.02 | 12.422 | 10.413 | 12.488 | 10.414 |
| 0.025 | 12.420 | 10.412 | 12.523 | 10.413 |
| 0.03 | 12.418 | 10.410 | 12.566 | 10.413 |
| 0.035 | 12.415 | 10.410 | 12.616 | 10.414 |
| 0.04 | 12.412 | 10.406 | 12.675 | 10.415 |
| 0.045 | 12.408 | 10.403 | 12.740 | 10.418 |
| 0.05 | 12.404 | 10.401 | 12.813 | 10.421 |

Table 8: Dispersion of the IPs with $\lambda$ for oxalic acid obtained using SC-QED-HF and F-SC-QED-HF and EOM-QED-CC and F-EOM-QED-CC

| $\lambda$ | SC-QED-HF | EOM-QED-CC | F-SC-QED-HF | F-EOM-QED-CC |
|---|---|---|---|---|
| 0.005 | 11.338 | 9.616 | 11.414 | 9.806 |
| 0.01 | 11.335 | 9.612 | 11.505 | 9.673 |
| 0.015 | 11.333 | 9.611 | 11.660 | 9.632 |
| 0.02 | 11.333 | 9.609 | 11.818 | 9.637 |
| 0.025 | 11.332 | 9.609 | 11.920 | 9.639 |
| 0.03 | 11.332 | 9.609 | 11.971 | 9.639 |
| 0.035 | 11.332 | 9.609 | 11.994 | 9.640 |
| 0.04 | 11.332 | 9.609 | 12.004 | 9.640 |
| 0.045 | 11.332 | 9.609 | 12.009 | 9.640 |
| 0.05 | 11.332 | 9.609 | 12.010 | 9.640 |

Table 9: Dispersion of the IPs with $\lambda$ for dimethyl ether obtained using SC-QED-HF and F-SC-QED-HF and EOM-QED-CC and F-EOM-QED-CC

| $\lambda$ | SC-QED-HF | EOM-QED-CC | F-SC-QED-HF | F-EOM-QED-CC |
|---|---|---|---|---|
| 0.005 | 10.914 | 9.583 | 10.917 | 9.579 |
| 0.01 | 10.913 | 9.582 | 10.926 | 9.578 |
| 0.015 | 10.913 | 9.581 | 10.942 | 9.577 |
| 0.02 | 10.912 | 9.580 | 10.964 | 9.577 |
| 0.025 | 10.910 | 9.579 | 10.993 | 9.576 |
| 0.03 | 10.909 | 9.577 | 11.027 | 9.576 |
| 0.035 | 10.907 | 9.575 | 11.068 | 9.576 |
| 0.04 | 10.905 | 9.572 | 11.115 | 9.577 |
| 0.045 | 10.903 | 9.569 | 11.168 | 9.579 |
| 0.05 | 10.900 | 9.566 | 11.228 | 9.582 |

Table 10: Dispersion of the IPs with $\lambda$ for urea obtained using SC-QED-HF and F-SC-QED-HF and EOM-QED-CC and F-EOM-QED-CC

| $\omega_c$ | SC-QED-HF | EOM-QED-CC | F-SC-QED-HF | F-EOM-QED-CC |
|---|---|---|---|---|
| 13.6 | 10.857 | 9.538 | 11.024 | 9.538 |
| 5.804 | 10.849 | 9.534 | 11.059 | 9.535 |
| 2.477 | 10.846 | 9.531 | 11.078 | 9.543 |
| 1.057 | 10.844 | 9.529 | 11.088 | 9.599 |
| 0.451 | 10.843 | 9.529 | 11.093 | 9.723 |
| 0.193 | 10.843 | 9.528 | 11.096 | 9.860 |
| 0.082 | 10.843 | 9.528 | 11.098 | 9.968 |
| 0.035 | 10.842 | 9.528 | 11.099 | 10.043 |
| 0.015 | 10.842 | 9.528 | 11.099 | 10.094 |
| 0.006 | 10.842 | 9.528 | 11.099 | 10.128 |
| 0.003 | 10.842 | 9.528 | 11.099 | 10.150 |

Table 11: Dispersion of the IPs with $\omega_c$ for hydrazine obtained using SC-QED-HF and F-SC-QED-HF and EOM-QED-CC and F-EOM-QED-CC

| $\omega_c$ | SC-QED-HF | EOM-QED-CC | F-SC-QED-HF | F-EOM-QED-CC |
|---|---|---|---|---|
| 13.6 | 11.981 | 10.401 | 12.014 | 10.402 |
| 5.804 | 11.974 | 10.396 | 12.051 | 10.400 |
| 2.477 | 11.969 | 10.393 | 12.140 | 10.410 |
| 1.057 | 11.966 | 10.392 | 12.295 | 10.472 |
| 0.451 | 11.965 | 10.391 | 12.452 | 10.606 |
| 0.193 | 11.964 | 10.391 | 12.553 | 10.752 |
| 0.082 | 11.964 | 10.390 | 12.603 | 10.866 |
| 0.035 | 11.964 | 10.390 | 12.626 | 10.946 |
| 0.015 | 11.963 | 10.390 | 12.636 | 10.999 |
| 0.006 | 11.963 | 10.390 | 12.640 | 11.034 |
| 0.003 | 11.963 | 10.390 | 12.642 | 11.057 |

Table 12: Dispersion of the IPs with $\omega_c$ for methanol obtained using SC-QED-HF and F-SC-QED-HF and EOM-QED-CC and F-EOM-QED-CC

| $\omega_c$ | SC-QED-HF | EOM-QED-CC | F-SC-QED-HF | F-EOM-QED-CC |
|---|---|---|---|---|
| 0.005 | 10.722 | 9.232 | 10.729 | 9.232 |
| 0.01 | 10.722 | 9.231 | 10.748 | 9.231 |
| 0.015 | 10.721 | 9.230 | 10.779 | 9.231 |
| 0.02 | 10.721 | 9.228 | 10.823 | 9.230 |
| 0.025 | 10.720 | 9.226 | 10.880 | 9.230 |
| 0.03 | 10.719 | 9.223 | 10.949 | 9.231 |
| 0.035 | 10.718 | 9.220 | 11.030 | 9.233 |
| 0.04 | 10.716 | 9.216 | 11.124 | 9.236 |
| 0.045 | 10.715 | 9.212 | 11.229 | 9.240 |
| 0.05 | 10.713 | 9.208 | 11.347 | 9.247 |

Table 13: Dispersion of the IPs with $\omega_c$ for formaldehyde obtained using SC-QED-HF and F-SC-QED-HF and EOM-QED-CC and F-EOM-QED-CC

| $\lambda$ | SC-QED-HF | EOM-QED-CC | F-SC-QED-HF | F-EOM-QED-CC |
|---|---|---|---|---|
| 0.005 | 10.722 | 9.232 | 10.729 | 9.232 |
| 0.01 | 10.722 | 9.231 | 10.748 | 9.231 |
| 0.015 | 10.721 | 9.230 | 10.779 | 9.231 |
| 0.02 | 10.721 | 9.228 | 10.823 | 9.230 |
| 0.025 | 10.720 | 9.226 | 10.880 | 9.230 |
| 0.03 | 10.719 | 9.223 | 10.949 | 9.231 |
| 0.035 | 10.718 | 9.220 | 11.030 | 9.233 |
| 0.04 | 10.716 | 9.216 | 11.124 | 9.236 |
| 0.045 | 10.715 | 9.212 | 11.229 | 9.240 |
| 0.05 | 10.713 | 9.208 | 11.347 | 9.247 |

Table 14: Dispersion of the IPs with $\lambda$ for alanine obtained using SC-QED-HF and F-SC-QED-HF and EOM-QED-CC and F-EOM-QED-CC

| $\omega_c$ | SC-QED-HF | EOM-QED-CC | F-SC-QED-HF | F-EOM-QED-CC |
|---|---|---|---|---|
| 13.6 | 11.133 | 10.206 | 11.153 | 10.205 |
| 5.804 | 11.132 | 10.204 | 11.185 | 10.204 |
| 2.477 | 11.132 | 10.204 | 11.264 | 10.209 |
| 1.057 | 11.133 | 10.204 | 11.404 | 10.239 |
| 0.451 | 11.133 | 10.205 | 11.547 | 10.320 |
| 0.193 | 11.133 | 10.205 | 11.639 | 10.421 |
| 0.082 | 11.133 | 10.206 | 11.684 | 10.505 |
| 0.035 | 11.133 | 10.207 | 11.705 | 10.565 |
| 0.015 | 11.133 | 10.208 | 11.714 | 10.607 |
| 0.006 | 11.133 | 10.209 | 11.718 | 10.634 |
| 0.003 | 11.133 | 10.210 | 11.720 | 10.653 |

Table 15: Dispersion of the IPs with $\omega_c$ for maleic acid obtained using SC-QED-HF and F-SC-QED-HF and EOM-QED-CC and F-EOM-QED-CC

| $\omega_c$ | SC-QED-HF | EOM-QED-CC | F-SC-QED-HF | F-EOM-QED-CC |
|---|---|---|---|---|
| 13.6 | 7.916 | 6.778 | 7.950 | 7.274 |
| 5.804 | 7.911 | 7.600 | 7.989 | 8.137 |
| 2.477 | 7.908 | 7.900 | 8.082 | 8.020 |
| 1.057 | 7.906 | 7.970 | 8.239 | 7.979 |
| 0.451 | 7.905 | 7.984 | 8.396 | 7.984 |
| 0.193 | 7.905 | 7.986 | 8.495 | 7.986 |
| 0.082 | 7.905 | 7.987 | 8.545 | 7.987 |
| 0.035 | 7.905 | 7.987 | 8.567 | 7.987 |
| 0.015 | 7.905 | 7.987 | 8.577 | 7.987 |
| 0.006 | 7.905 | 7.987 | 8.582 | 7.987 |
| 0.003 | 7.905 | 7.987 | 8.583 | 7.987 |

Table 16: Dispersion of the IPs with $\omega_c$ for pyrrole obtained using SC-QED-HF and F-SC-QED-HF and EOM-QED-CC and F-EOM-QED-CC

| $\omega_c$ | SC-QED-HF | EOM-QED-CC | F-SC-QED-HF | F-EOM-QED-CC |
|---|---|---|---|---|
| 13.6 | 11.064 | 9.597 | 11.098 | 9.598 |
| 5.804 | 11.056 | 9.593 | 11.135 | 9.595 |
| 2.477 | 11.050 | 9.589 | 11.225 | 9.603 |
| 1.057 | 11.047 | 9.588 | 11.381 | 9.655 |
| 0.451 | 11.046 | 9.587 | 11.537 | 9.776 |
| 0.193 | 11.045 | 9.586 | 11.636 | 9.910 |
| 0.082 | 11.045 | 9.586 | 11.685 | 10.01 |
| 0.035 | 11.044 | 9.586 | 11.708 | 10.09 |
| 0.015 | 11.044 | 9.586 | 11.718 | 10.14 |
| 0.006 | 11.044 | 9.586 | 11.722 | 10.17 |
| 0.003 | 11.044 | 9.586 | 11.723 | 10.19 |

Table 17: Dispersion of the IPs with $\omega_c$ for glycine obtained using SC-QED-HF and F-SC-QED-HF and EOM-QED-CC and F-EOM-QED-CC
